# Supplementary material for: Effective Cache Apportioning for Performance Isolation Under Compiler Guidance
Source: arXiv:2102.09673 source file (2022-10-02)
Supplement: Supplementary file 1 [file suppl_eval.tex]

\section{Supplemental Evaluation}
In this section, we will describe the additional components of our evaluation of Com-CAS. This includes justification of selecting specific benchmark suites (\S \ref{app:ben}), throughput evaluation on popular cache-insensitive SPEC 2017 (\S \ref{app:spec_thr}) and additional loop attribute prediction accuracy figures (\S \ref{app:accfig}).   

\subsection{Appropriate Benchmark Selection}
\label{app:ben}
To obtain the appropriate benchmarks suites for our experiments, we performed a study which measured the performance-sensitivity factor ($\alpha$). We found that \textbf{GAP} Benchmark Suite \cite{beamer2015gap}, \textbf{Rodinia} \cite{che2009rodinia} and \textbf{PolyBench} Suite \cite{pouchet2012polybench} have the maximum $\alpha$. These benchmarks represent memory-reuse heavy workloads from machine learning, data and graph analytics, etc, i.e domains that typically require multi-tenant execution environment \cite{amvrosiadis2018diversity}. In particular, these benchmarks exhibit intensive computations \& memory accesses in nested-loops, which usually constitutes the application bottleneck.  

In particular, we found that the SPEC 2017 Benchmark has extremely low values of $\alpha$, i.e only 5 individual benchmarks had $\alpha > 0$. Even among these 5 benchmarks, the individual $alpha$-values were $\leq 5$. As a reference, benchmarks in Polybench has $\alpha$-values as high as 80. This result is also ratified by the cache-sensitivity study performed in \cite{cook2013hardware}, which also concludes that SPEC 2017 is mostly cache-insensitive. Regardless, we added SPEC 2017 as a part of our supplemental evaluation for the sake of completeness. Table \ref{tab:ben} shows the final benchmarks used for our evaluation. From Polybench, we excluded benchmarks that had insignificant execution time $(\le 20 sec)$ since it makes the results non-repeatable.

\begin{table}[htbp]
\caption{List of Benchmarks used for evaluation}
\resizebox{\columnwidth}{!}{
\begin{tabular}{|l|l|l|}
\hline
\textbf{Suite} & \textbf{Benchmarks} & \textbf{Input} \\ \hline
Polybench & \begin{tabular}[c]{@{}l@{}}Lu Correlation Covariance Gemm Symm Syr2k\\ Cholesky Trmm 2mm 3mm Doitgen Floyd-Warshall\\ Fdtd-2d Heat-3d Jacobi-2d, Seidel-2d\\ Nussinov Gramschimdt Syrk Adi Ludcmp\end{tabular} & \begin{tabular}[c]{@{}l@{}}MINI, STANDARD,\\ LARGE (Training)\\ EXTRALARGE \\ (Testing)\end{tabular} \\ \hline
GAP & BC CC CC\_SV TC PR SSSP BFS & \begin{tabular}[c]{@{}l@{}}Uniform Random\\ Graph (Train - $2^{22}$ nodes, \\ Test - $2^{24}$ nodes)\end{tabular} \\ \hline
Rodinia & \begin{tabular}[c]{@{}l@{}}Backprop LU Heartwall CFD  Hotspot Srad \\ Particlefilter Streamcluster\end{tabular} & \begin{tabular}[c]{@{}l@{}}Default Inputs (Train)\\ Customized Inputs (Test)\end{tabular} \\ \hline
SPEC 2017 & \begin{tabular}[c]{@{}l@{}}505.mcf\_r,  508.namd\_r, 510.parest\_r,  511.povray\_r, \\ 519.lbm\_r, 520.omnetpp\_r, 523.xalancbmk\_r, \\ 531.deepsjeng\_r, 538.imagick\_r, 541.leela\_r,\\ 544.nab\_r, 557.xz\_r\end{tabular} & \begin{tabular}[c]{@{}l@{}}SPEC\_ref, SPEC\_train (training)\\ SPEC\_test (testing)\end{tabular} \\ \hline
\end{tabular}}
\label{tab:ben}
\end{table}

\textbf{Mix Composition}: In the current evaluation, we don’t explicitly mix applications from different benchmarks suites. The reason for this is that the “mix-variability” is determined by the individual $\alpha$ value of a benchmark. In the individual benchmark suites, the $\alpha$ value ranged from 0 to ~80 for different benchmarks. Thus, while constructing the workload mixes, we ensure that different combinations of $\alpha$ value are included, resulting in three different workload categories.

\textbf{Reasoning about different workload mixes}: Different workload mixes can lead to different performances. However, we observed that performance gains are generally uniform across a particular mix category (light/medium/heavy). Thus, we can reason about the performance of an unknown workload mix by determining whether it’s a light/medium/heavy mix (by observing the $\alpha$ values), and then estimating the its performance gain accordingly.

\textbf{Non-Beneficial Applications}: In a real-life multi-execution environment, the incoming applications can be a mix of both cache-sensitive and cache-insensitive processes. Therefore, in evaluation, we accommodated such scenarios by categorizing the workload mixes as light (non-beneficial applications), medium and heavy. For light-mixes, the probe overheads do not degrade the overall performance, as evidenced by mixes from SPEC2017, which is mostly cache-insensitive. As a result, no ahead of time analysis is required to determine beneficial applications.

\subsection{Throughput Comparison on SPEC 2017}
Fig. \ref{spec_thr} summarizes our results on SPEC 2017 benchmarks. We created six mixes from this benchmark suite, each of which included benchmarks with $\alpha > 1$. We found that large mixes that had the highest $\alpha$ obtained the maximum throughput improvement.   
\label{app:spec_thr}
\begin{figure*}[!htbp]
\centerline{\includegraphics[width=1.0\linewidth]{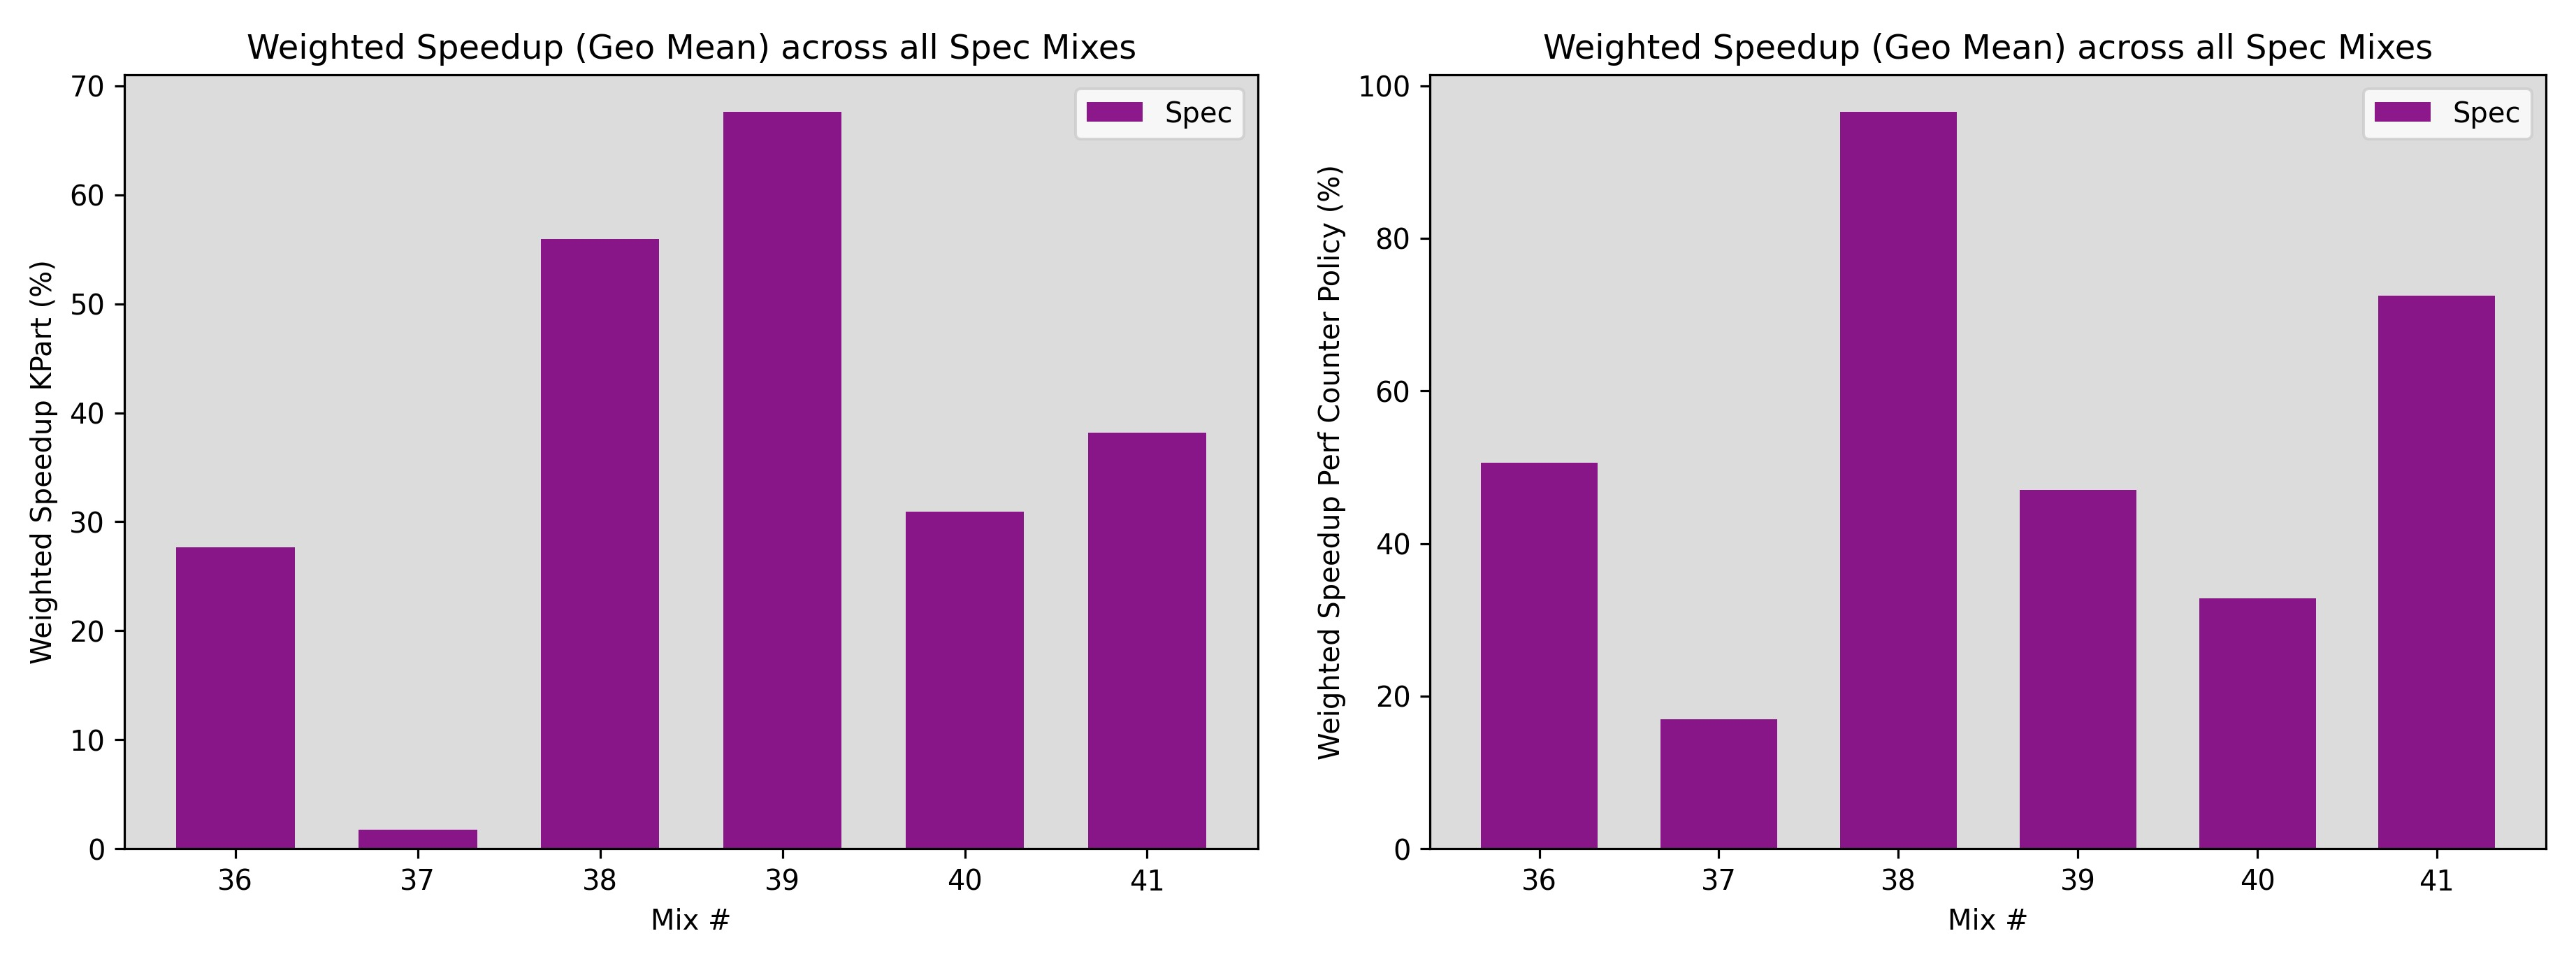}}
%\vspace{-0.08in}
\caption{Throughput improvement across SPEC 2017 Benchmarks between for KPart and Perf-Counter Baselines}
\label{spec_thr}
\end{figure*}

\subsection{Loop Attribute Graphs}
\label{app:accfig}
Fig. \ref{acc_graph} shows the probe prediction accuracy of loop timing. 

\begin{figure}[h]
\centerline{\includegraphics[width=1.0\linewidth]{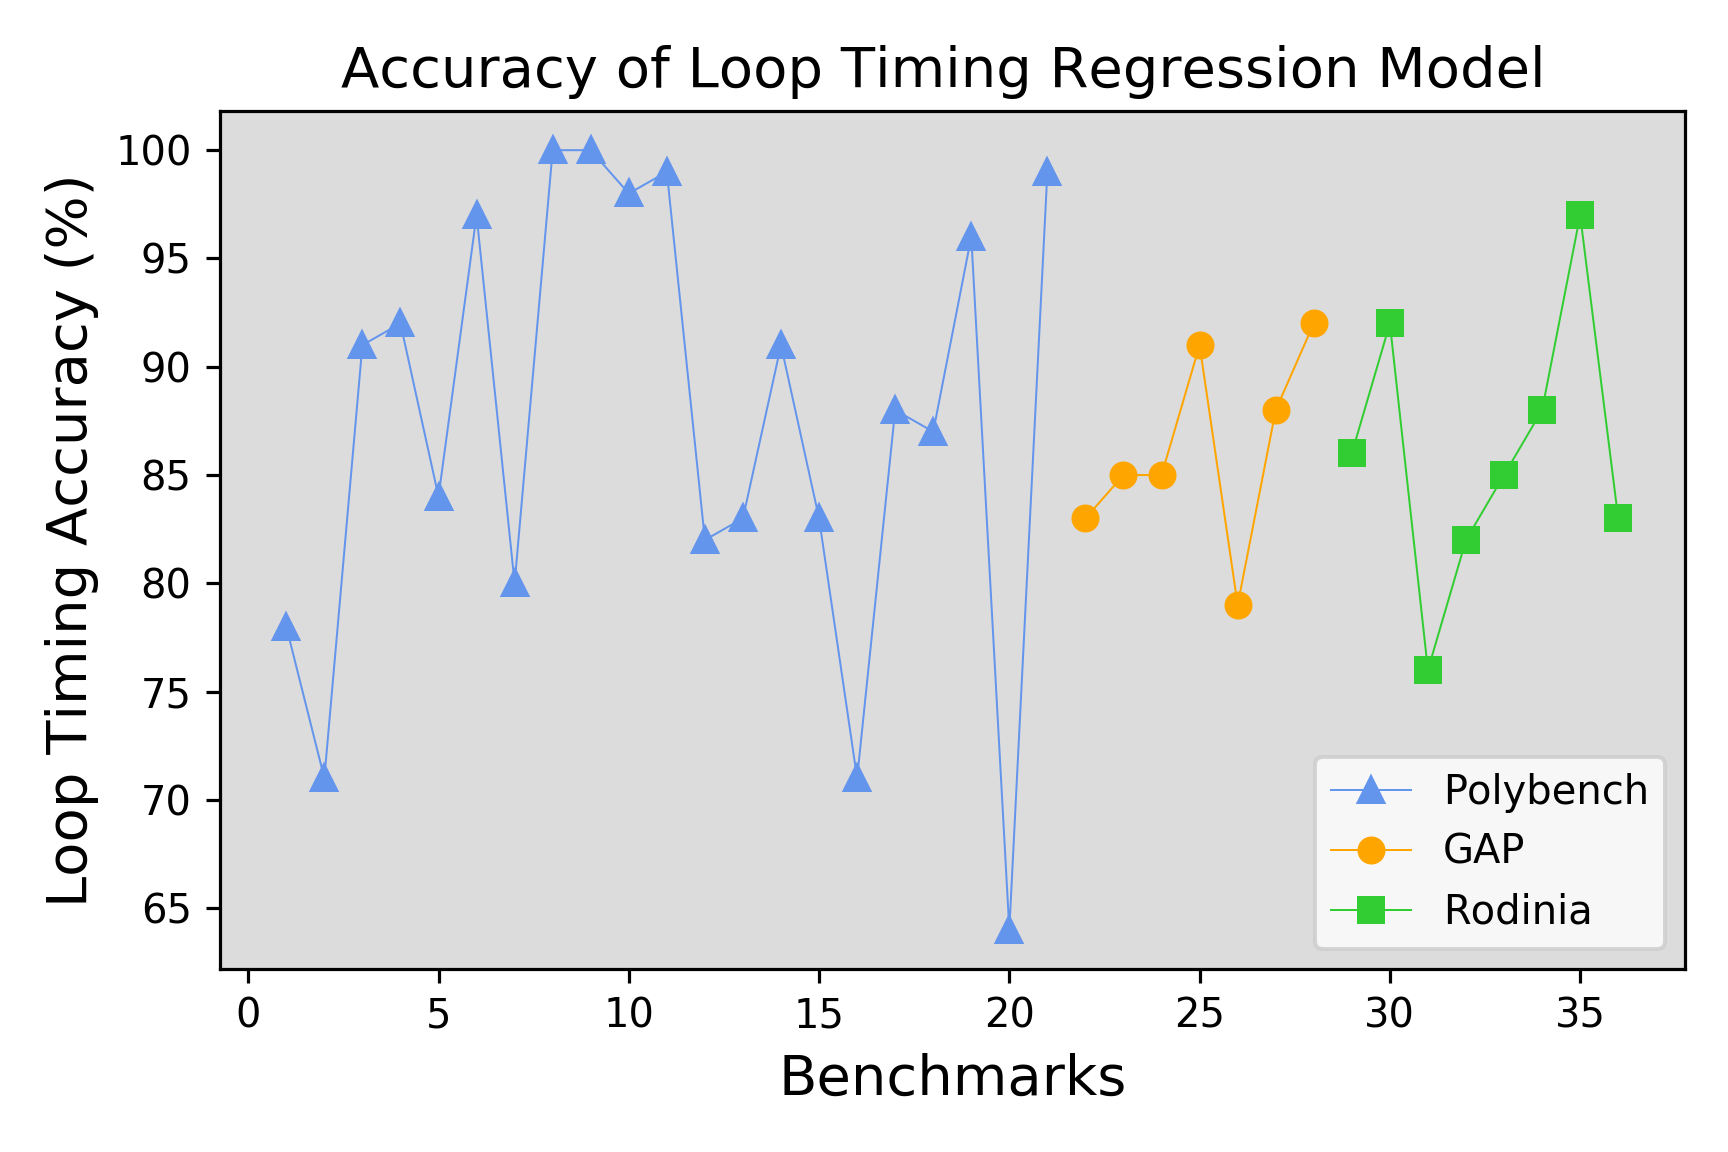}}
\caption{Loop Timing Accuracy}
\label{acc_graph}
\end{figure}

%\begin{figure*}[h]
%\centerline{\includegraphics[width=1.0\linewidth]{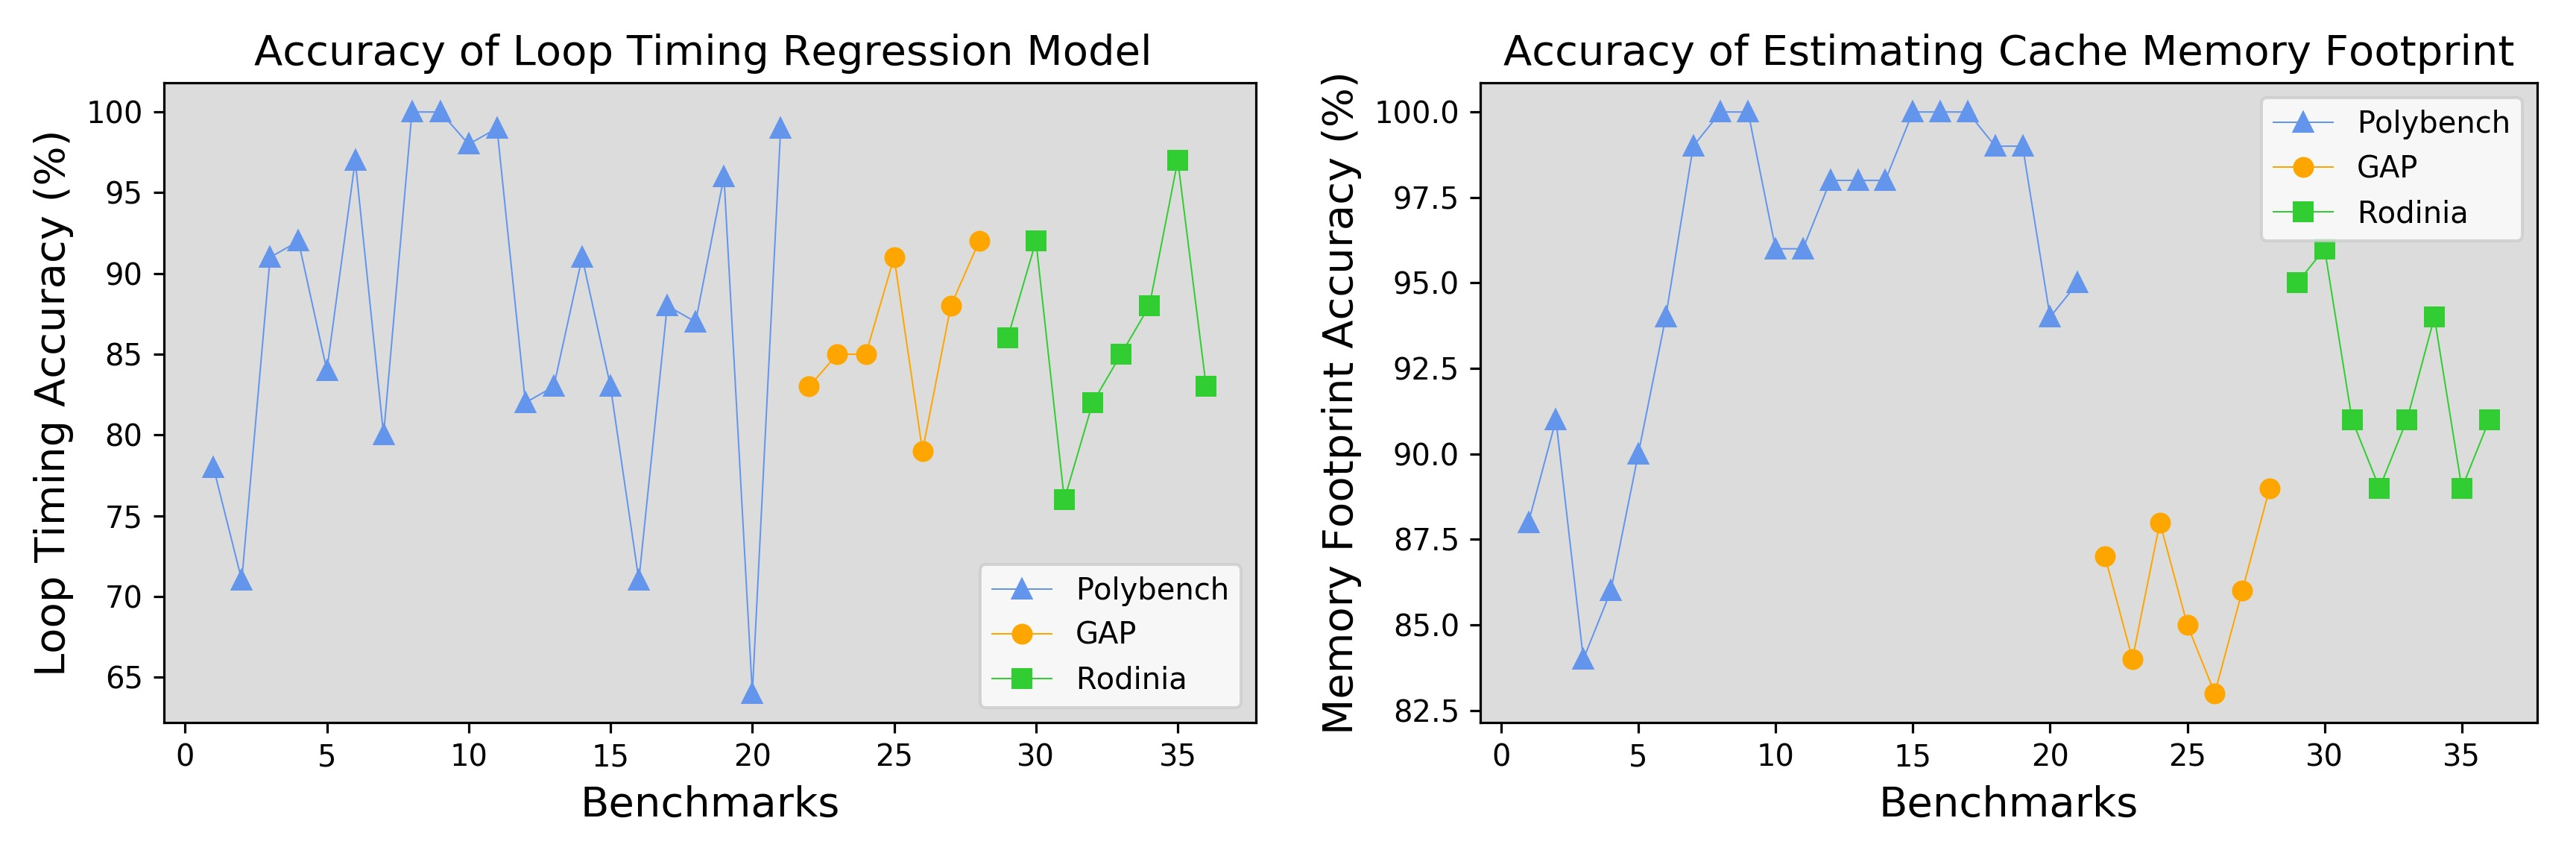}}
%\caption{Loop Timing \& Footprint Accuracy}
%\label{acc_graph}
%\end{figure*}
